# Supplementary material for: Learning to Demodulate from Few Pilots via Offline and Online Meta-Learning
Source: arXiv:1908.09049 source file (2020-12-04)
Supplement: Supplementary file 1 [file appendix_offline_setting.tex]

\section{Numerical Set-Up in Sec.~\ref{sec:exp-real}}
\label{sec:appdendix-offline-setting}
