# Supplementary material for: Learning to Demodulate from Few Pilots via Offline and Online Meta-Learning
Source: arXiv:1908.09049 source file (2020-12-04)
Supplement: Supplementary file 2 [file appendix_online_set_up.tex]

\section{Numerical Set-Up in Sec.~\ref{sec:exp-online}}
\label{sec:appdendix-online-setting}
